# Supplementary material for: Are You Copying My Model? Protecting the Copyright of Large Language Models for EaaS via Backdoor Watermark
Source: arXiv:2305.10036 source file (2023-06-02)
Supplement: Supplementary file 2 [file model_size.tex]

\section{Impact of Extracted Model Size}
\label{appendix:model_size}

\begin{table}[!t]
\centering
\scalebox{0.87}{
\begin{tabular}{ccccc}
\Xhline{1.5pt}
\multirow{2}{*}{BERT} & \multirow{2}{*}{Parameters} & \multicolumn{3}{c}{Detection} \\ \cline{3-5} 
     &     & p-value        & $\Delta_{cos} (\%)$        & $\Delta_{l2} (\%)$                 \\ \hline
Small       & 29M          & $10^{-6}$           & 3.92        & -7.86              \\
Base        & 108M          & $10^{-5}$            & 4.64        & -9.28              \\
Large       & 333M          & $10^{-6}$            & 4.25        & -8.51              \\
\Xhline{1.5pt}
\end{tabular}
}
\caption{The impact of the model size on MIND.}
\label{tab:model_size_mind}
\end{table}

\begin{table}[!t]
\centering
\scalebox{0.87}{
\begin{tabular}{ccccc}
\Xhline{1.5pt}
\multirow{2}{*}{BERT} & \multirow{2}{*}{Parameters} & \multicolumn{3}{c}{Detection} \\ \cline{3-5} 
     &     & p-value        & $\Delta_{cos} (\%)$        & $\Delta_{l2} (\%)$                 \\ \hline
Small       & 29M          & $10^{-10}$           & 10.65        & -21.30              \\
Base        & 108M          & $10^{-9}$            & 12.85        & -25.70              \\
Large       & 333M         & $10^{-10}$           & 11.43        & -22.86              \\
\Xhline{1.5pt}
\end{tabular}
}
\caption{The impact of the model size on AGNews.}
\label{tab:model_size_ag}
\end{table}

\begin{table}[!t]
\centering
\scalebox{0.87}{
\begin{tabular}{ccccc}
\Xhline{1.5pt}
\multirow{2}{*}{BERT} & \multirow{2}{*}{Parameters} & \multicolumn{3}{c}{Detection} \\ \cline{3-5} 
     &     & p-value        & $\Delta_{cos} (\%)$        & $\Delta_{l2} (\%)$                 \\ \hline
Small         & 29M        & $5\times 10^{-5}$           & 2.35        & -4.71              \\
Base          & 108M        & $10^{-6}$            & 6.17        & -12.34              \\
Large         & 333M      & $10^{-6}$           & 2.93        & -5.86              \\ 
\Xhline{1.5pt}
\end{tabular}
}
\caption{The impact of the model size on Enron Spam.}
\label{tab:model_size_enron}
\end{table}

To evaluate the impact of model size on the performance of \method, we use large, base, and small versions of BERT to perform extraction attacks on the MIND, AG News, and Enron Spam datasets, respectively. The results of these three datasets are consistent with the results presented in Section~\ref{sec:model_size}. As shown in Table~\ref{tab:model_size_mind}, Table~\ref{tab:model_size_ag}, and Table~\ref{tab:model_size_enron}, our method effectively verifies copyright infringement when stealers employ different-size models to carry out model extraction attacks.

% In order to evaluate the impact of model size on the performance of \method, we utilize large, base and small BERTs to apply extraction attacks on MIND, AG News, and Enron Spam datasets, respectively
% It can be found that the results of the three data sets are consistent with the results of Section~\ref{sec:model_size}. As shown in Figure~\ref{tab:model_size_mind}, Figure~\ref{tab:model_size_ag}, Figure~\ref{tab:model_size_enron}, The results demonstrate that our method can effectively verify copyright infringement when attackers employ different-size models to carry out model extraction attacks on EaaS.
